# Supplementary material for: Security and Privacy of IP-ICN Coexistence: A Comprehensive Survey
Source: arXiv:2209.02835 source file (2023-07-11)
Supplement: Supplementary file 1 [file discussion-additional-technologies.tex]

\begin{table*}[!ht] 
%\tiny
\centering
%\caption{Evaluation of S\&P features for coexistence architectures}
\caption{Summary of the additional technologies used for each deployment approach.}
\label{tab:additional-technologies}
    \begin{tabular}{ c c c  c  c c c c c c c}
      \toprule
      %\hline
       \makecell{\multirow{3}{*}{Deployment approach}} &
       \multirow{3}{*}{\makecell{Analysed \\ architectures}} &
       \multicolumn{5}{c}{Deployment scenario} &
       \multicolumn{4}{c}{Additional technologies} \\
       \cline{3-11}\\
       & & \makecell{ICN-ICN \\ in IP} & \makecell{ICN-IP \\ in IP} & \makecell{ICN-IP \\ in ICN} & \makecell{IP-IP \\ in ICN} & \makecell{Border \\ Island} & \makecell{SDN} & \makecell{CDN} & \makecell{DTN} & \makecell{NFV} \\
      \toprule 
       \makecell{Overlay} & 10 & 10 & 4 & 0 & 0 & 0 & 6 & 0 & 0 & 0 \\
        \midrule
        \makecell{Underlay} & 6 & 4 & 4 & 3 & 3 & 4 & 2 & 2 & 1 & 1\\
        \midrule
        \makecell{Hybrid} & 4 & 3 & 3 & 3 & 3 & 2 & 0 & 0 & 0 & 0 \\
        
    \bottomrule
    \end{tabular}
\end{table*}
